# Supplementary material for: Understanding and Improving the Role of Projection Head in Self-Supervised Learning
Source: arXiv:2212.11491 source file (2022-12-22)
Supplement: Supplementary file 1 [file appendix.tex]

\section*{Appendix}
\label{sec:Appendix}
